# Supplementary material for: Scalable Neural Network Training over Distributed Graphs
Source: arXiv:2302.13053 source file (2024-02-11)
Supplement: Supplementary file 1 [file communication.tex]

\section{Communication Cost}
\label{appdx:comm}

\subsection{GNN}
In a typical message-passing GNN all the layers of the model are trained together. As a result, in a single epoch, each train and validation client requires the features and intermediate embeddings of its neighbors and need to send back gradients to them. Only the features of the neighbors can be cached by a client as rest of it keeps changing in every epoch. In each training round, only a small set of clients get the model from the server for training and validation tasks. Therefore, the clients in the $\num$-hop of neighborhood of these clients need the model too. Server being unacquainted by the neighborhood of any client, an efficient way to provide models to the neighborhood of train and validation clients is through train-clients only. So, in every round, a client upon receiving the model from the server, either for training or validation, propagates it in its $\num$ hop neighborhood. Eventually, sending and receiving models, embeddings and gradients contribute to the client-to-client communication of training GNNs in federated setup. Client-to-server communication include the cost to receive the model in a round for training and send back the gradients to aggregate.

\subsection{\toolgnn }
Following the training procedure for \toolgnn as described in \ref{sec:retexo-train}. Each train and validation node requires embeddings from the previously trained model. It might be the case that the node selected for a round or any other node in its $\num$ hop neighborhood doesn't has the previously trained model. To avoid such situation, server performs a sync i.e. send the trained model after finishing training for each model in \toolgnn to every node. Such a sync is unreasonable for layers in case of GNNs as it will increase the communication cost significantly. Similar to the features in the case of GNNs, In \tool every node can cache the embeddings of its neighbors after every model as it will remain same throughout the training process. In our implementation, after the sync from the server, each compute its embeddings on the latest model and share it among all it neighbors before the start of the training of next model. Finally, only sharing of embeddings after every model except last contribute to the client-to-client communication of training \toolgnn in federated setup. For client-to-server channel, it includes the cost to receive models and send back gradients in a round and some additional cost to sync the latest trained model after training each model. Still the total cost over client-to-server is significantly lesser than in case of GNNs because of the reduced size of models in \toolgnn.
