# Supplementary material for: Scalable Neural Network Training over Distributed Graphs
Source: arXiv:2302.13053 source file (2024-02-11)
Supplement: Supplementary file 2 [file gcn-train.tex]

\section{Distributed \gcn Learning}
\label{appdx:gcn-learning}

In each training round, the server sub-samples a set of nodes from all available train-clients and assigns training and validation tasks to them. For training a $2$-layer \gcn, here we detail the actions performed during the message-passing round by the client that received the training task.

% \server The server distributes the model parameters $\fc{f}_\theta$ to the train-clients ($\Gamma[\set{V}]\subset \set{V}$) that are ready to participate in that round of training. 

\subsection{Message Passing}
\paragraph{First representations} The train-client $v$ sends its first representation $\arr{Q}^0_v$ and the \gcn's first layer $\theta^0_{IH}$ to its neighbors $u\in \set{N}(v)$. The neighbors of the train-client will do two things. First, they will reply to the train-client with their own first representation $\arr{Q}^0_u$. Second, they will request their neighbors to share their first representations with them so that they can compute their second representation $\arr{Q}^1_u$. The $2$-hop neighbors of the train-client will then reply with their first representations.

\paragraph{Second representations} Once the train-client and its neighbors receive the necessary first representations, they will start computing their second representation using the model.

\begin{align*}
\arr{Q}^1_v &= \sigma(\frac{1}{\cf{deg}(v)}\cdot \sum_{u}\arr{Q}^{0}_u\cdot\arr{\theta}^0_{IH})\\
\arr{Q}^1_u &= \sigma(\frac{1}{\cf{deg}(u)}\cdot \sum_{u'}\arr{Q}^{0}_{u'}\cdot\arr{\theta}^0_{IH})\text{, } u'\in\set{N}(u)\text{, }u\in \set{N}(v)
\end{align*}

The train-client's neighbors will send their second representations to the train-client. The train-client can then compute the final representation, i.e., the node embeddings. 

\begin{align*}
    \arr{Q}^2_v = \sigma(\frac{1}{\cf{deg}(v)}\cdot \sum_{u}\arr{Q}^{1}_u\cdot\arr{\theta}^1_{HO})
\end{align*}

% training clients sends its second representation to its neighbors and asks its neighbors to respond with their own second representations. However, notice that the neighbors of the training client have to ask their neighbors to send them their first representations to compute their own second representation. So, they ask their neighbors ($2$-hop neighbors of training clients $v$) to send them their first representations. The neighbors of the training clients then compute their second representation.

Similarly, if the \gcn had $\num$-layers then all the nodes in the $\num$-hop neighborhood will participate in the message passing. The nodes at a distance of $p$ will compute $0^{th}$ to ${\num-p}$ representations.

\subsection{Gradient Computation}

\client Each training client $v$ will compute the loss and gradients with respect to the parameters. However, notice that the weights are shared between the nodes and their neighbors. For the shared parameters, the gradient computation would require additional factors, i.e., a real-valued array representing neighbor's input to the shared weights during the forward pass, from the neighbors. A train-client will have to ask its neighbors to provide the necessary factors. Therefore, the gradients can only be computed with another round of message passing. The factors are dependent on the model architecture. In a \gcn, the first layer parameters are shared. Therefore, for each neighbor of the train-client, it will have to ask the input to that layer used by its neighbor during the forward pass. Therefore, the size of factors required from a neighbor is the size of the input to that layer. For a $\num$-layer \gcn, these factors would come from $(\num-1)$-hop neighbors. The message passing is conducted similar to the one during the forward pass.

% At the end of the message passing, each train-client will update the model based on a pre-decided learning rate and send their local models to the server. The server will aggregate the local models and use it to start the next round.

\subsection{Model Aggregation}

Each sampled train-client ($v$) will locally update the model based with learning rate $\eta$.

 \begin{align*}
     \fc{f}'_{\theta}[v] = \fc{f}_{\theta}[v] - \eta\cdot\frac{\partial L_{v}}{\partial \theta}
 \end{align*}

All sampled clients for training share their updated model with the server. The server will aggregate the locally updated models and use it to start the next round.

% \server The server will receive all updated models which then computes the aggregated model. The server will share this aggregated model in the next round of the learning process.

% \begin{align*}
%     \fc{f}'_{\theta} = \sum_{v}{\fc{f}'_{\theta}[v]}\text{, }v\in\Gamma{\set{V}}
% \end{align*}
