# Supplementary material for: Scalable Neural Network Training over Distributed Graphs
Source: arXiv:2302.13053 source file (2024-02-11)
Supplement: Supplementary file 3 [file tool-train.tex]

\section{Training \toolgnn}
\label{appdx:tooltrain}

\begin{algorithm}[t]
% \SetAlgoLined
% \SetKwInOut{Input}{Input}
% \SetKwInOut{Output}{Output}
\caption{$\cf{FederatedLearning}$: Outline of the federated learning protocol to train an \mlp in \toolgnn}
\label{alg:fl}
\begin{algorithmic}[1]
\STATE {\bfseries Input:} Server, Clients, message-passing round number: $\hopiter$, \# training rounds: $R$

\textit{// initialize server and clients}
\STATE {Server:} \{$\set{V}$, $\set{V}^{tr}$, $\set{V}^{val}$, $\set{V}^{test}$, $\fc{f}_{\theta}$, $\num$, $\numrounds$\}
\STATE {Clients:} [\{$v$, $nei$:$\set{N}(v)$, $feat$:$\arr{F}[v]$, $label$:$\arr{L}[v]$, $Opt$\} $\forall v \in [|\set{V}|]$]
\item[]\item[]
\textit{//To train model number m} 
\STATE {\bfseries Server executes:}
    \STATE\hspace*{\myindent} $\text{\mlp}_m$ = $\fc{f}^{\hopiter-1}_{\theta}$
    \STATE\hspace*{\myindent} $\cf{initModel}(\text{\mlp}_m)$ \textit{// initialize the model}
    \item[]
    \begin{ALC@g}
        \FOR{$i=0$ to $i=R-1$}
            \STATE $\set{V}^{tr}_s, \set{V}^{val}_s=\cf{sampleNodes}(\set{V}^{tr}, \set{V}^{val})$ \textit{// sample sets of training and validation clients}
            \STATE $\cf{sendMessage}(\set{V}^{tr}_s, \text{\mlp}_m, \text{``train''})$
            \STATE $\cf{sendMessage}(\set{V}^{val}_s, \text{\mlp}_m, \text{``validation''})$
            \item[]
            \STATE $\text{\mlp}^j_m$, $client_j$ = $\cf{receiveMessage()}$ \textit{// wait for the replies from all clients}
            \item[]
            \STATE // On receiving all updated local models
            \STATE $\text{\mlp}^{agg}_m = \frac{\sum_{j=0}^{j=|\set{V}^{tr}_s|} \text{\mlp}^{j}_m}{|\set{V}^{tr}_s|}$
            \STATE$\text{\mlp}_m = \text{\mlp}^{agg}_m$
        \ENDFOR
    \end{ALC@g}
    \STATE\hspace*{\myindent} {\bfseries Output:}{Trained $\text{\mlp}_m$}
\item[]
\STATE {\bfseries Each client executes:}
    \STATE\hspace*{\myindent} $\text{\mlp}_m, task$ = $receiveMessage()$
    % \bindent
    \begin{ALC@g}
        \IF{$task$ is \text{``train''}}
            \STATE $\text{\mlp}^{tr}_m = \cf{trainModel}(\text{\mlp}_m, feat, label, Opt)$
            \STATE $\cf{sendMessage}(server, \text{\mlp}^{tr}_m)$
        \ENDIF
    \end{ALC@g}
    \STATE \hspace*{\myindent}\textit{// for validation compute accuracy and send it back}
\end{algorithmic}
\end{algorithm}
\begin{algorithm}[t]
\caption{$\cf{AsyncMessagePassing}$: Outline of message-passing round to train \toolgnn}
\label{alg:messagep}
\begin{algorithmic}[1]
\STATE {\bfseries Input:} Clients, $timeout$, message-passing round number: $\hopiter$
\STATE {Clients:} [\{$v$, $nei$:$\set{N}(v)$, $feat$:$\arr{F}[v]$, $label$:$\arr{L}[v]$, $Opt$\} $\forall v \in [|\set{V}|]$\}]

\item[]\item[]
\textit{// For message-passing round number m}
\STATE {\bfseries Each client ($v$) executes:}
    \STATE\hspace*{\myindent} $Q^m$ = $\cf{computeEmbedding(m)}$ \textit{// Computes $m^{th}$ embedding}
    \begin{ALC@g}
        \WHILE{not $timeout$}
            \STATE\textit{// scan for available client-to-client communication channels}
            \STATE $clients\_available$ = $\cf{scanForClients()}$ 
            \item[]
            \FOR{$u$ in $clients\_available$}
                \IF{$u \in \set{N}(v)$}
                    \STATE $conn$ = $\cf{initConnection(u)}$
                    \STATE \textit{// send and receive embeddings}
                    \STATE $conn.\cf{sendEmbedding}(Q^m)$
                    \STATE $Q_u^m$ = $conn.\cf{recvEmbedding()}$
                    \STATE $conn.close()$ \textit{// close connection}
                \ENDIF
            \ENDFOR
        \ENDWHILE
    \end{ALC@g}
%     \begin{ALC@g}
%         \FOR{$u$ in $\set{N}(v)$}
        
%         \ENDFOR
%     \end{ALC@g}
%     \ENDWHILE
% \FOR{$client$ in Clients}
%     \STATE \textit{// Computes $m^{th}$ embedding}
%     \STATE $client.Q^m$ = $\cf{client.computeEmb(m)}$
% \ENDFOR

% \WHILE{not $timeout$}
%     \FOR{$client$ in Clients}
%         \FOR{$client\_nei$ in $client.neighbors$}
%             \STATE \textit{// if $client$ \& $client\_nei$ are in proximity}
%             \IF{$\cf{Contact}(client, client\_nei)$}
%                 \STATE \textit{send and receive embeddings}
%                 \STATE $client.\cf{sendEmbedding}(client\_nei, client.Q^m)$
%             \ENDIF
%         \ENDFOR
%     \ENDFOR
% \ENDWHILE
\end{algorithmic}
\end{algorithm}

We provide more detailed algorithms for federated learning and message-passing rounds to train \toolgnns in Algorithms~\ref{alg:fl} and~\ref{alg:messagep} respectively.

\subsection{Federated Learning}
\label{appdx:toolfl}

We use the $\cf{FedSGD}$ protocol to train every \mlp in \toolgnn. The server knows all the clients, and which ones to use for training, validation, and testing (Line $2$ in Algorithm~\ref{alg:fl}). The clients locally store their own feature vector, label, and their neighbors (Line $3$ in Algorithm~\ref{alg:fl}).  The clients have access to the optimizer used for training too. In practice, the server can send the optimizer, with a fresh internal state, to the clients before training a model. As the training of the model goes by, each client's optimizer's internal state changes locally until the training is completed. Finally, the clients will locally store their neighbors' embeddings from all previous message-passing rounds.

Consider a scenario where the server wants to train the model $\text{\mlp}_m$, i.e., the $m^{th}$ \mlp. The server will first initialize the model (Lines $5$-$6$). For each training round, the server will sample a set of clients, from the set of train-clients, for training and another for validation. The server then sends a message to these clients along with the most recent state of the model and the task that clients have to perform (Lines $8$-$10$). On receiving this message from the server, each client proceeds to execute the requested task (Line $18$). If a client is requested to train the model then the client will perform one forward-pass and one backward-pass on the model. It will update the model based on the learning rate, weight decay and the momentum, as given by the optimizer's internal state. The client will then return the updated local model to the server (Lines $19$-$21$). If a client is requested to validate the model then the client just evaluates the model on its feature vector and lets the server know if the predicted label is correct.

The server waits for the updated local models from the sampled clients. On receiving all of them, the server will proceed to aggregate the models and start a new round of training with that model (Lines $11$-$14$).~\footnote{The $\cf{FedSGD}$ protocol can be modified to handle asynchronous and unreliable networks too~\cite{nguyen2022federated}.} The number of training rounds can be fixed beforehand, based on the budget available, or the training can be stopped early by tracking the validation accuracy.

\subsection{Asynchronous Message Passing}
\label{appdx:mp}

The server initiates a message-passing round before training an \mlp (except for the first one) by sending the latest updated model to all the clients. For instance, if the server wants to train $\text{\mlp}_m$ then it will first send all the clients $\text{\mlp}_{m-1}$ and ask the clients to start the message-passing round. The clients will use its own features, embeddings, neighbors' embeddings from previous message-passing rounds, and previously trained models to compute the current embedding $Q^m$ (Line $5$). The client then shares this embedding with its neighbors (Lines $9$-$14$) when the communication channels are available. For instance, in proximity networks, the sharing happens whenever they are in proximity. In distributed social networks, the sharing happens whenever the neighbors are online and a successful connection with them is established.
